# Supplementary material for: AI and ethics in insurance: a new solution to mitigate proxy discrimination in risk modeling
Source: arXiv:2307.13616 source file (2023-07-25)
Supplement: Supplementary file 1 [file appendix_logit.tex]

\section{Reminder on the logistic regression}
\label{appendix:logistic regression}
\paragraph{} This section gives a quick reminder about the logistic regression \cite{butucea22}. A binary logistic model is used to model the probability of a certain class: $Y \in \{0,1\}$0. The model assumes that the outcomes conditioned on the explanatory variables follow a Bernoulli distribution:
\begin{equation*}
    Y_j|X_j^{(1)}=x_j^{(1)},\dots,X_j^{(n)}=x_j^{(n)} \sim \mathcal{B}(p_j)
\end{equation*}
with $p_j=\mathbb{P}(Y_j=1|X_j^{(1)}=x_j^{(1)},\dots,X_j^{(n)}=x_j^{(n)})$
and that the $logit$ of this probability is modelled as a linear combination of the n explanatory variables:
\begin{equation*}
    \begin{split}
        logit(\mathbb{P}(Y_j=1|X_j^{(1)}=x_j^{(1)},\dots,X_j^{(n)}=x_j^{(n)})) & =b_0+b_1x_j^{(1)}+\dots+b_nx_j^{(n)} \\
         & =\textbf{B}\cdot\bm{x_j}
    \end{split}
\end{equation*}
with $\textbf{B}=(b_0,\dots,b_n)$ and $\bm{x_j}=(1,x_j^{(1)},\dots,x_j^{(n)})^T$ \\
As a reminder,
\begin{equation*}
    logit(p)=ln(\frac{p}{1-p}), p \in (0,1)
\end{equation*}
and 
\begin{equation*}
    logit^{-1}(x)=\frac{1}{1+e^{-x}}, x \in \mathbb{R}
\end{equation*}
The vector $\textbf{B}$ is estimated by maximizing the log-likelihood. The likelihood of an independently and identically distributed sample of size $J$ is
\begin{equation*}
    \begin{split}
        L & =\mathbb{P}(Y_1=y_1,\dots,Y_J=y_J|X^{(1)}=x^{(1)},\dots,X^{(n)}=x^{(n)}) \\
         & =\prod_{j=1}^J \mathbb{P}(Y_j=y_j|X_j^{(1)}=x_j^{(1)},\dots,X_j^{(n)}=x_j^{(n)}) \\
         & =\prod_{j=1}^J \frac{1}{1+e^{-(b_0+b_1x_j^{(1)}+\dots+b_nx_j^{(n)})}}
    \end{split}
\end{equation*}
We can then find the $\bm{\hat{B}}$ that maximizes log(L) and classify a new individual j by applying Bayes' rule:
\begin{equation*}
    \begin{split}
        Y_j=1 & \iff \mathbb{P}(Y_j=1|\bm{X_j}=\bm{x_j})>\mathbb{P}(Y_j=0|\bm{X_j}=\bm{x_j}) \\
         & \iff \mathbb{P}(Y_j=1|\bm{X_j}=\bm{x_j})>\frac{1}{2} \\
         & \iff \frac{1}{1+e^{-\bm{\hat{B}}\cdot\bm{x_j}}}>\frac{1}{2} \\
         & \iff \bm{\hat{B}}\cdot\bm{x_j}>0
    \end{split}
\end{equation*}
So
\begin{equation*}
    Y_j=\mathbb{1}_{\bm{\hat{B}}\cdot\bm{x_j}>0}
\end{equation*}

\newpage
